# Supplementary material for: Deep learning of fMRI big data: a novel approach to subject-transfer decoding
Source: arXiv:1502.00093 source file (2015-01-31)
Supplement: Supplementary file 1 [file caption.tex]

\label{fig:appendix_psa}
PSMs of the other classes.
See the caption of Fig.\,\ref{fig:PSA} for the specification.
