# Supplementary material for: Deep learning of fMRI big data: a novel approach to subject-transfer decoding
Source: arXiv:1502.00093 source file (2015-01-31)
Supplement: Supplementary file 2 [file size.tex]

width=700
